# Supplementary material for: IGL-Bench: Establishing the Comprehensive Benchmark for Imbalanced Graph Learning
Source: arXiv:2406.09870 source file (2025-03-01)
Supplement: Supplementary file 1 [file 7_rebuttal.tex]

\section{{Revision for Rebuttal}}
\label{app:rebuttal}

\subsection{{Revision for Section~\ref{sec:res_rq1_node_class} and Appendix~\ref{sec:add_rq1_node_class}}}
\subsubsection{{Table~\ref{tab:main_res_node_cls_acc_20} (Revised)}}
\input{table/main_res_node_cls_acc_20_rbt}

\newpage
\subsubsection{{Table~\ref{tab:res_node_cls_acc_all} (Revised)}}
\input{table/res_node_cls_acc_all_rbt}

\newpage
\subsubsection{{Table~\ref{tab:res_node_cls_bacc_all} (Revised)}}
\input{table/res_node_cls_bacc_all_rbt}

\newpage
\subsubsection{{Table~\ref{tab:res_node_cls_mf1_all} (Revised)}}
\input{table/res_node_cls_mf1_all_rbt}

\newpage
\subsubsection{{Table~\ref{tab:res_node_cls_auc_all} (Revised)}}
\input{table/res_node_cls_auc_all_rbt}

\newpage
\subsection{{Revision for Section~\ref{sec:res_rq1_node_global_topo} and Appendix~\ref{sec:add_rq1_node_global_topo}}}
\subsubsection{{Table~\ref{tab:main_res_node_topo_acc_2_high} (Revised)}}
\input{table/main_res_node_topo_acc_2_high_rbt}

\subsubsection{{Table~\ref{tab:res_node_topo_acc_all} (Revised)}}
\input{table/res_node_topo_acc_all_rbt}

\newpage
\subsubsection{{Table~\ref{tab:res_node_topo_bacc_all} (Revised)}}
\input{table/res_node_topo_bacc_all_rbt}

\subsubsection{{Table~\ref{tab:res_node_topo_mf1_all} (Revised)}}
\input{table/res_node_topo_mf1_all_rbt}

\newpage
\subsubsection{{Table~\ref{tab:res_node_topo_auc_all} (Revised)}}
\input{table/res_node_topo_auc_all_rbt}

\newpage
\subsection{Additional results for Table~\ref{tab:res_node_cls_mf1_all}}
\input{table/rbt_perf1_cora}
\input{table/rbt_perf1_citeseer}
\input{table/rbt_perf1_pubmed}
\input{table/rbt_perf1_computer}
\input{table/rbt_perf1_photo}
\input{table/rbt_perf1_arxiv}
\input{table/rbt_perf1_chameleon}
\input{table/rbt_perf1_squirrel}
\input{table/rbt_perf1_actor}
